# Supplementary material for: Can Language Model Agents be Helpful Circuit Explainers in Mechanistic Interpretability?
Source: arXiv:2606.24026 source file (2026-09-02)
Supplement: Supplementary file 1 [file appendix-human-judge.tex]

\section{Human Annotation}
\label{app:human-judge}
We conduct human annotation to validate the reliability of the LLM-judged metrics used in our evaluation. The annotation covers two judged metrics: role description quality ($Q_{\text{desc}}$), derived task accuracy ($Acc_{\text{task}}$). We additionally collect human annotations for validation plan soundness ($S_{\text{val}}$) and hypothesis grounding as process-level diagnostics.

\par For $Q_{\text{desc}}$, $Acc_{\text{task}}$, and $S_{\text{val}}$, the annotation was performed by two human annotators (CS Graduate students with experience in ML).

\paragraph{Annotation instructions.}
Both annotators were given a standardized annotation \texttt{README}, detailed metric definitions, and representative examples for each score level. The instructions followed the same evaluation rubrics used for the LLM-judge evaluation. The annotators worked independently, and LM backbone identities were hidden and randomized. Annotators used a Streamlit-based interface that presented one
benchmark task at a time. For each task, the interface first
showed the task context, including the ground-truth task summary, up to five input-output examples, and the list of localized components with their ground-truth tags. For each localized component, annotators then evaluated the outputs of two \agent backbones, displayed as Agent A and Agent B. The underlying backbone identities were hidden from annotators and randomized to reduce bias.

For each agent-component pair, annotators first saw the agent's
hypothesis and validation plan as a read-only context. They then
rated validation-plan soundness ($S_{\text{val}}$) as
\textit{Sound}, \textit{Partial}, or \textit{Unsound}. A
\textit{Sound} plan directly tests the key mechanistic prediction of the hypothesis; a \textit{Partial} plan is causally relevant but indirect or incomplete; and an \textit{Unsound} plan does not meaningfully test the hypothesis.

Annotators next saw the ground-truth tag and role note for the
component, followed by the agent's predicted role description. The agent's predicted tag was shown only as context and was not itself rated. Annotators rated role description quality
($Q_{\text{desc}}$) as \textit{Correct}, \textit{Partial}, or
\textit{Wrong}. A \textit{Correct} description captures the
component's task-specific role; a \textit{Partial} description
captures the main role but is vague, incomplete, or contains an incorrect mechanistic sub-claim; and a \textit{Wrong}
description contradicts the reference role or describes a
different function.

Finally, at the bottom of each task, annotators saw the
ground-truth task summary and each agent's derived task
description. They rated the task description accuracy
($Acc_{\text{task}}$) as \textit{Correct} or \textit{Wrong},
indicating whether the derived description recovered the
task-level behavior. Annotators could optionally provide a short
rationale for each rating. The hidden mapping from Agent A/B to
the underlying \agent backbone was recorded automatically for
analysis but was not visible during annotation.
\paragraph{Agreement computation.}
For ordinal 3-point metrics ($Q_{\text{desc}}$ and
$S_{\text{val}}$), we report linearly weighted Cohen's $\kappa$.
Linear weighting is appropriate because adjacent disagreements,
such as 1 vs. 2, are less severe than endpoint disagreements,
such as 0 vs. 2. For binary $Acc_{\text{task}}$, we report ordinary Cohen's $\kappa$ without weighting.

We report inter-annotator agreement on the larger GPT/Claude subset: Agreement is \textbf{almost perfect} for $Q_{\text{desc}}$ and $Acc_{\text{task}}$, with Cohen's $\kappa$ of 0.8 and 0.96, respectively. Agreement is \textbf{moderate} for $S_{\text{val}}$ ($\kappa=0.46$) due to the subjective nature of the metric.

\begin{table}[h]
\centering
\small
\begin{tabular}{lcc}
\toprule
Metric & $n$ & $\kappa$ \\
\midrule
\multicolumn{3}{l}{\textbf{Human--human agreement}} \\
\midrule
$Q_{\text{desc}}$ & 110 & 0.802 \\
$S_{\text{val}}$  & 110 & 0.460 \\
$Acc_{\text{task}}$ & 62 & 0.963 \\
\midrule
\multicolumn{3}{l}{\textbf{Lower human vs. Lower judge agreement}} \\
\midrule
$Q_{\text{desc}}$ & 110 & 0.753 \\
$S_{\text{val}}$  & 110 & 0.481 \\
$Acc_{\text{task}}$ & 62 & 0.864 \\
\bottomrule
\end{tabular}
\caption{
Human--human inter-annotator agreement and Human--LLM-judge agreement on the larger GPT/Claude annotation subset. The value of $n$ counts model-output instances, $\kappa$ denotes linearly weighted Cohen's $\kappa$ for ordinal metrics.
}
\label{tab:human-iaa-large}
\end{table}

\paragraph{Per-judge agreement with each annotator.}
Table~\ref{tab:per-judge-iaa} reports linearly-weighted Cohen's
$\kappa$ between each LLM judge (GPT-5.4, Gemini-3.1-Pro) and each human annotator on the 10-task / 17-components subset used for the main-text human validation ($n=68$ component-level instances for $Q_{\text{desc}}$,
$S_{\text{val}}$ and $n=40$ task-level for $Acc_{\text{task}}$).
The two judges track both annotators at moderate-to-substantial
agreement on $Q_{\text{desc}}$ and $Acc_{\text{task}}$
($\kappa \geq 0.62$). On $S_{\text{val}}$, Gemini is closer to
both annotators than GPT, which is systematically stricter on
validation plans. This asymmetry is what motivates the
conservative min-aggregation we use in the main results.

\begin{table}[h]
\centering
\small
\begin{tabular}{l c c c c}
\toprule
Metric & A-GPT & A-Gemini & B-GPT & B-Gemini \\
\midrule
$Q_{\text{desc}}$  & 0.73 & 0.78 & 0.63 & 0.74 \\
$S_{\text{val}}$   & 0.23 & 0.59 & 0.43 & 0.49 \\
$Acc_{\text{task}}$& 0.73 & 0.74 & 0.73 & 0.74 \\
\bottomrule
\end{tabular}
\caption{Linear-weighted Cohen's $\kappa$ between each LLM judge
and each human annotator (A, B) on the cross-backbone subset
($n=68$ for $Q_{\text{desc}}/S_{\text{val}}$, $n=40$ for
$Acc_{\text{task}}$).}
\label{tab:per-judge-iaa}
\end{table}

\paragraph{Annotation for Hypothesis grounding.}
We additionally annotate hypothesis grounding as a process-level
diagnostic. This annotation was performed by one human annotator (CS Graduate Student) on the 10-task, 17-component subset used for the main-text human validation. For each \agent backbone and each component, the annotator was shown the natural-language observation produced by the agent and the subsequent hypothesis generated from that observation, along with the task context (i.e. task description, examples, and ground truth component roles). The annotator judged whether the hypothesis was supported by the observation on a 3-point scale: 0 if the hypothesis contradicted or ignored the observation, 1 if it was partially supported but added unsupported details, and 2 if it was fully supported by the observation. This metric evaluates whether the agent's hypothesis follows from its own observed evidence. It
does not directly evaluate whether the hypothesis matches the
ground-truth component role.
